# Supplementary material for: Inferring synchronizability of networked heterogenous oscillators with machine learning
Source: arXiv:2303.03107 source file (2023-02-11)
Supplement: Supplementary file 1 [file Supplementary.pdf]

Supplementary Material for  
**Inferring synchronizability of networked heterogenous  
oscillators with machine**

Liang Wang, Huawei Fan, Yafeng Wang, Jian Gao,  
Yueheng Lan, Jinghua Xiao, and Xingang Wang

Corresponding author: X. G. Wang (wangxg@snnu.edu.cn)

**CONTENTS**

|                                                                           |    |
|---------------------------------------------------------------------------|----|
| I. FNN technique                                                          | 2  |
| II. Properties of optimal allocation                                      | 4  |
| III. Results for scale-free network                                       | 5  |
| IV. Results for Nepal power-grid                                          | 7  |
| V. Results for cat-brain network                                          | 8  |
| VI. Results for Nematode neuronal network                                 | 10 |
| VII. Results for chaotic Rössler oscillators                              | 11 |
| VIII. Results for chaotic Foodweb oscillators                             | 12 |
| IX. Inferring the synchronization performance of a new set of oscillators | 14 |
| X. Impacts of training data on machine performance                        | 15 |

## I. FNN TECHNIQUE

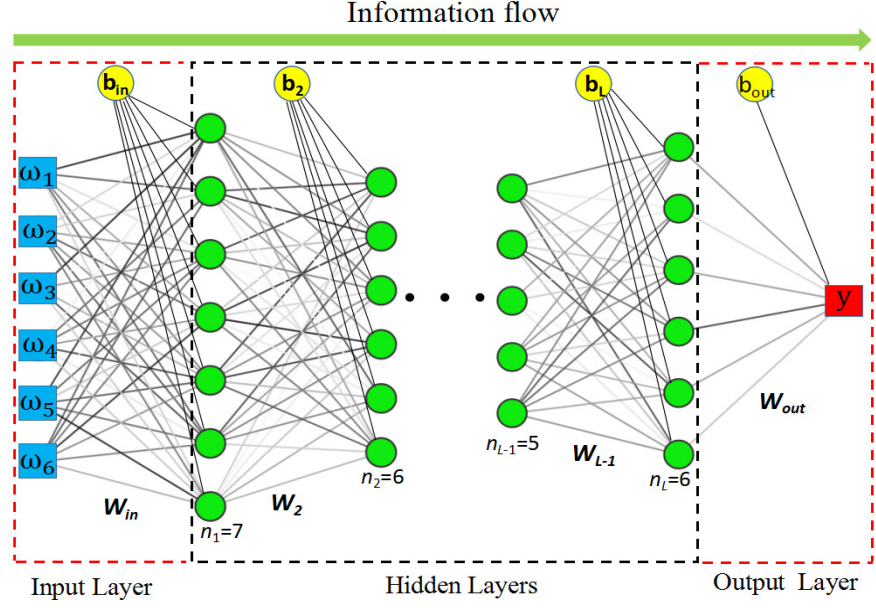

FIG. S1. *Schematic of FNN.* The FNN adopted in the present study consists of three layers: an input layer,  $L$  hidden layers, and an output layer. The input data is  $\Omega = [\omega_1, \dots, \omega_N]^T$ , which denotes a specific allocation scheme of the oscillators on the network. (As illustration, here we set  $N = 6$ .) The output is the scalar  $y$ , which could be either the critical coupling for synchronization or the synchronization order parameter. The neighboring layers are coupled by the all-to-all fashion, and information is propagated from the input layer to the output layer in a one-way fashion. The hyperparameters of FNN include  $L$  and the size of each hidden layer,  $\{n_h\}$ ,  $h = 1, \dots, L$ . The model parameters to be trained from the measured data include the weights of all network connections ( $\mathbf{W}_{in}, \mathbf{W}_{h=2, \dots, L-1}, \mathbf{W}_{out}$ ) and the bias vectors ( $\mathbf{b}_{in}, \mathbf{b}_{h=2, \dots, L-1}, b_{out}$ ).

The feed-forward neural network (FNN) is the type of artificial neural network wherein information is propagated along the layered nodes in one direction. Inspired by the way how neurons are processing information in the human brain, a FNN contains a large number of hypothetical neurons, which process the inputting information by a nonlinear activation function. Different from the neurons in the brain, nodes in FNN normally do not have intrinsic dynamics, and therefore their states are determined completely by their input signals. A typical FNN consists of three modules: an input layer, a series of hidden layers, and an output layer. Nodes within the same layer are not connected, but nodes in the neighboring layers are globally coupled (i.e., each node in the next layer receives inputting signals from all nodes in the previous layer). The coupling relationship of the nodes are fixed, but the weights of the couplings,  $(\mathbf{W}_{in}, \mathbf{W}_{h=2, \dots, L-1}, \mathbf{W}_{out})$ , are to be trained from the measured data. Another set of parameters to be trained from the measured data are the bias vectors  $(\mathbf{b}_{in}, \mathbf{b}_{h=2, \dots, L-1}, b_{out})$ . The input data is a specific allocation scheme of the oscillators and is represented by the vector  $\Omega = [\omega_1, \dots, \omega_N]$ . The output is a scalar denoted as  $y$ . Depending on the inference tasks, the output can be the critical coupling for the network to achieve synchronization or the synchronization order parameter under a specific coupling strength. A schematic diagram showing the structure of FNN is plotted in Fig. S1.

For the fixed network structure (determined by the hyperparameters) and model parameters

(including the coupling matrices and the bias vectors), the state of the FNN is updated as follows. First, the state of the first hidden layer,  $\mathbf{x}_1 \in \mathbb{R}^{n_1}$ , is updated by the operation

$$\mathbf{x}_1 = f(\mathbf{W}_{in}\mathbf{\Omega} + \mathbf{b}_{in}), \quad (\text{S1.1})$$

where  $\mathbf{W}_{in} \in \mathbb{R}^{n_1 \times N}$  is the input matrix,  $\mathbf{\Omega} = [\omega_1, \dots, \omega_N]^T$  is the vector denoting the oscillator allocation, and  $\mathbf{b}_{in} \in \mathbb{R}^{n_1}$  is the input bias vector. In Eq. (S1.1),  $f(x)$  is the activation function. In the current study, unless otherwise specified, we adopt the rectified linear activation function (ReLU) to update the nodes:  $f(x) = x$  for  $x > 0$ , and  $f(x) = 0$  for  $x \leq 0$  (for its advantages on simulating efficiency, prevention of gradient disappearance and overfitting, etc). The signals are then propagated to other hidden layers in sequence as

$$\mathbf{x}_h = f(\mathbf{W}_h\mathbf{x}_{h-1} + \mathbf{b}_h), \quad (\text{S1.2})$$

where  $h = 2, \dots, L$  is the index of the hidden layers,  $\mathbf{x} \in \mathbb{R}^{n_h}$  is the state vector of the  $h$ th hidden layer,  $\mathbf{W}_h \in \mathbb{R}^{n_h \times n_{h-1}}$  is the coupling matrix between hidden layers  $h-1$  and  $h$ ,  $n_h$  is the size of the  $h$ th hidden layer, and  $\mathbf{b}_h \in \mathbb{R}^{n_h}$  is the bias vector for the  $h$ th hidden layer. After the signals have been propagated to the  $L$ th hidden layer, the machine output is generated by the operation

$$y = f(\mathbf{W}_{out}\mathbf{x}_L + b_{out}), \quad (\text{S1.3})$$

where  $y$  is the output scalar,  $\mathbf{W}_{out} \in \mathbb{R}^{1 \times n_L}$  is the output matrix, and  $b_{out}$  is the output bias.

In what follows, we take the inference of the critical coupling,  $\epsilon^p$ , for phase synchronization as an example to demonstrate the implementation of FNN. In this application, the measured data (obtained by model simulations) are of the form  $(\Omega_l, \epsilon_l^p)$ , with  $\Omega_l$  the  $l$ th allocation scheme of the oscillators and  $\epsilon_l^p$  the critical coupling where the synchronization order parameter,  $r$ , exceeds the threshold  $r_c = 0.9$  for the  $l$ th allocation scheme.  $\tilde{M} = 800$  data points are obtained in total. As each data point requires a simulation on the variation of  $r$  with respect to  $\epsilon$ ,  $\tilde{M} = 800$  synchronization transitions have been simulated. The measured data are divided into two sets by random. The first set contains  $M = 500$  data points, which will be used in the training phase for obtaining the model parameters; the second set contains  $M' = 300$  data points, which will be used in the validation phase for optimizing the machine hyperparameters.

In the training phase, we input the allocation schemes,  $\{\Omega_l\}_{l=1}^M$ , individually, and generate the corresponding outputs,  $\{y_l\}_{l=1}^M$ , according to Eqs. (S1.1-S1.3). The mission of the training is to obtain the set of model parameters (i.e., the coupling matrices and bias vectors) such that the outputs given by the machine are as close as possible to the true values, i.e.,  $y_l \approx \epsilon_l^p$  for  $l = 1, \dots, M$ . This is equivalent to finding the minimum value of the loss function

$$E = \frac{1}{2} \sum_{l=1}^M (y_l - \epsilon_l^p)^2, \quad (\text{S1.4})$$

by tuning the model parameters. In the current work, the search of the minimum loss function is accomplished by the gradient-descent back propagation algorithm, as follows. Starting from a set of random model parameters, we calculate the machine outputs,  $\{y_l\}_{l=1}^M$ , according to Eqs. (S1.1-S1.3), and then the loss function  $E$ . We next introduce small random perturbations to the initial model parameters, and calculate again the loss function based on the new machine outputs. Based on the loss functions and the perturbations, we update the model parameters by the increments

$$\Delta \tilde{\mathbf{W}} = -\eta \frac{\partial E}{\partial \tilde{\mathbf{W}}}, \Delta \tilde{\mathbf{b}} = -\eta \frac{\partial E}{\partial \tilde{\mathbf{b}}}, \quad (\text{S1.5})$$

in which  $\eta$  is the learning rate,  $\tilde{\mathbf{W}} = (\mathbf{W}_{in}, \mathbf{W}_{h=2,\dots,L-1}, \mathbf{W}_{out})$  and  $\tilde{\mathbf{b}} = (\mathbf{b}_{in}, \mathbf{b}_{h=2,\dots,L-1}, b_{out})$  are the model parameters. As a balance between searching speed and accuracy, here we set the learning rate as  $\eta = 0.001$ . We adopt the adaptive moment estimation (ADAM) strategy in TensorFlow to speed up the searching process.

In the validation phase, by fixing the model parameters, we generate by the trained machine the critical couplings for allocations in the validation set containing  $M' = 300$  data points. The performance of the machine on the validation dataset is also evaluated by the loss function  $E$ . The value of  $E$  is dependent on the hyperparameters,  $L$  and  $\{n_h\}$ ,  $h = 1, \dots, L$ , and the set of hyperparameters giving the minimum  $E$  is defined as the optimal ones. In our current study, we adopt the strategy of Bayesian optimization to find the optimal hyperparameters (please see Ref. [23] in the manuscript and the references therein). Once the optimal hyperparameters are obtained, the validation phase is completed.

Finally, in the prediction phase, by the optimal hyperparameters obtained in the validation phase and the model parameters obtained in the training phase, we choose a new random allocation scheme (neither included in the training dataset nor included in the validation dataset) as the input, and predict by the machine the critical coupling,  $\epsilon^p$ , for this new allocation to reach phase synchronization. This is done for  $K = 1000$  random allocations in total. By the same set of allocations, we obtain by simulation the true critical couplings where  $r > r_c = 0.9$ , and then compare the true results with the ones predicted by the machine, which gives the averaged prediction error quantifying the machine performance, i.e., the quantity  $\langle e^p \rangle$  in the main text.

A similar process is also applied in inferring the critical coupling,  $\epsilon^f$ , for frequency synchronization and the synchronization order parameter,  $r$ , under a specific coupling strength (within the transition regime). In inferring  $\epsilon^f$ , the total number of measured data points is also  $\tilde{M} = 800$ , among which  $M = 500$  data points are used for training the model parameters and  $M' = 300$  points are used for optimizing the hyperparameters ( $L = 1$  and  $n_1 = 100$ ). In inferring  $r$  for the intermediate coupling strength  $\epsilon = 1.2$ , the total number of data points obtained by simulations is  $\tilde{M} = 1000$ , among which  $M = 700$  data points are used for training the model parameters and  $M' = 300$  points are used for optimizing the hyperparameters [ $L = 3$  and  $(n_1, n_2, n_3) = (150, 200, 50)$ ]. Still, the prediction performance is evaluated by averaging over  $K = 1000$  random allocations, which give  $\langle e^f \rangle$  (for frequency synchronization) and  $\langle e \rangle_r$  (for synchronization order parameter).

## II. PROPERTIES OF OPTIMAL ALLOCATION

In the study of synchronization optimization through oscillator allocation on complex network of coupled heterogenous phase oscillators, some common features have been observed in the optimal allocation schemes (see, for instance, Refs. [14,19] in the main text), including: (1) a positive correlation between the node degree and the natural frequency; (2) a negative correlation between the frequencies of the neighboring nodes. These features are also observed in the optimal allocation scheme identified by the machine in the current study. Shown in Fig. S2(a) is the degree-frequency correlation of the ( $m = 10$ ) relocatable nodes in the optimal allocation that the machine has identified among  $K = 10000$  random candidates. (The synchronization performance of the optimal allocation is shown in Fig. 2 in the main text.) We see that the correlation is weakly positive (the fitted slope is about 0.02). As a comparison, we plot in Fig. S2(a) also the degree-frequency correlation for a random allocation scheme (case 1 in Fig. 1 of the main text), in which the fitted slope is about  $-0.01$ . We see that the degree-frequency correlation of the

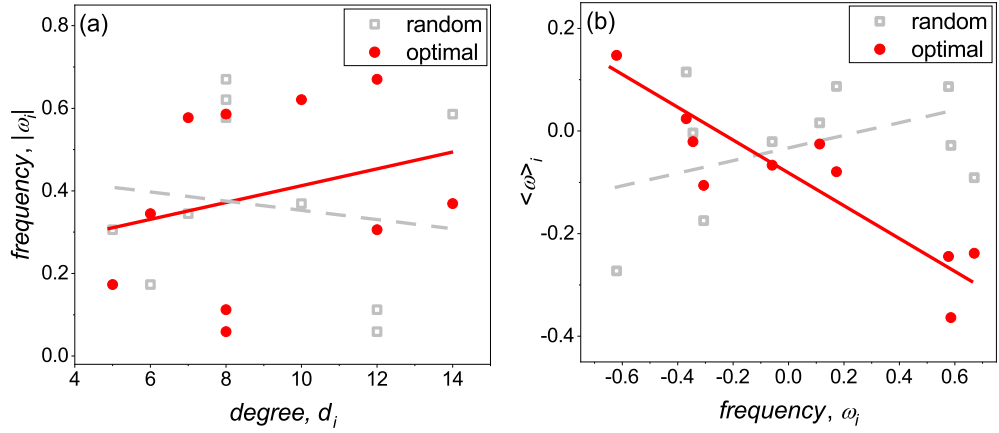

FIG. S2. For the network model studied in the manuscript, the properties of the optimal allocation identified by the machine. (a) The relationship between the natural frequency  $|\omega_i|$  and the node degree  $d_i$ . The fitted slope is about 0.02. (b) The relationship between the averaged natural frequencies  $\langle \omega_i \rangle$  of the neighboring nodes and the natural frequency  $\omega_i$  of node  $i$ . The fitted slope is about  $-0.33$ . Gray squares are the results for a random allocation (case 1 in Fig. 1 in the manuscript), in which the degree and frequency is negatively correlated (the fitted slope is about  $-0.01$ ), and the frequency-frequency correlation is positive (the fitted slope is about 0.1).

optimal allocation is clearly different from that of the random allocation. Shown in Fig. S2(b) is the correlation between the natural frequency of node  $i$ ,  $\omega_i$ , and the averaged natural frequency of its neighboring nodes,  $\langle \omega_i \rangle = \sum_{j=1}^N \mathbf{A}_{ij} \omega_j / d_i$ , with  $\mathbf{A}$  the adjacency matrix and  $d_i$  the node degree. We see that the frequencies are negatively correlated, with the fitted slope being about  $-0.33$ . We plot in Fig. S2(b) also the frequency-frequency correlation for the random allocation, which shows that the frequencies are positively correlated (the fitted slope is about 0.1).

The results in Fig. S2 are obtained for the scenario of constrained allocation, in which the network size is  $N = 20$  and only  $m = 10$  oscillators are relocatable. The correlation properties could be more distinct by considering large-size complex networks and more relocatable oscillators (e.g.,  $N \sim 1000$  and  $m \sim 500$ ). The properties of the optimal allocation for large-size complex networks requires large-scale simulations, which are out of our computational ability at present.

### III. RESULTS FOR SCALE-FREE NETWORK

The scale-free network is generated by the BA algorithm, as follows. First a core of 5 globally connected nodes is generated, then at each time step of the network evolution one new node is introduced, which is connected to 5 existing nodes by the mechanism of preferential attachment (see Ref. [1] in the manuscript). The final network contains  $N = 100$  nodes and 485 links. Different from the random network studied in the manuscript, in scale-free network there exist some large-degree nodes, namely the hub nodes, which play a vital role on the network synchronization performance. Still, we adopt the model of networked heterogeneous phase oscillators, with the natural frequencies of the oscillators being chosen randomly within the range  $(-1, 1)$ . Again, we consider the scenario of constrained allocation. Specifically, we first assign all oscillators on the network by random, and then choose  $m = 10$  oscillators by the order of node degree (i.e., the

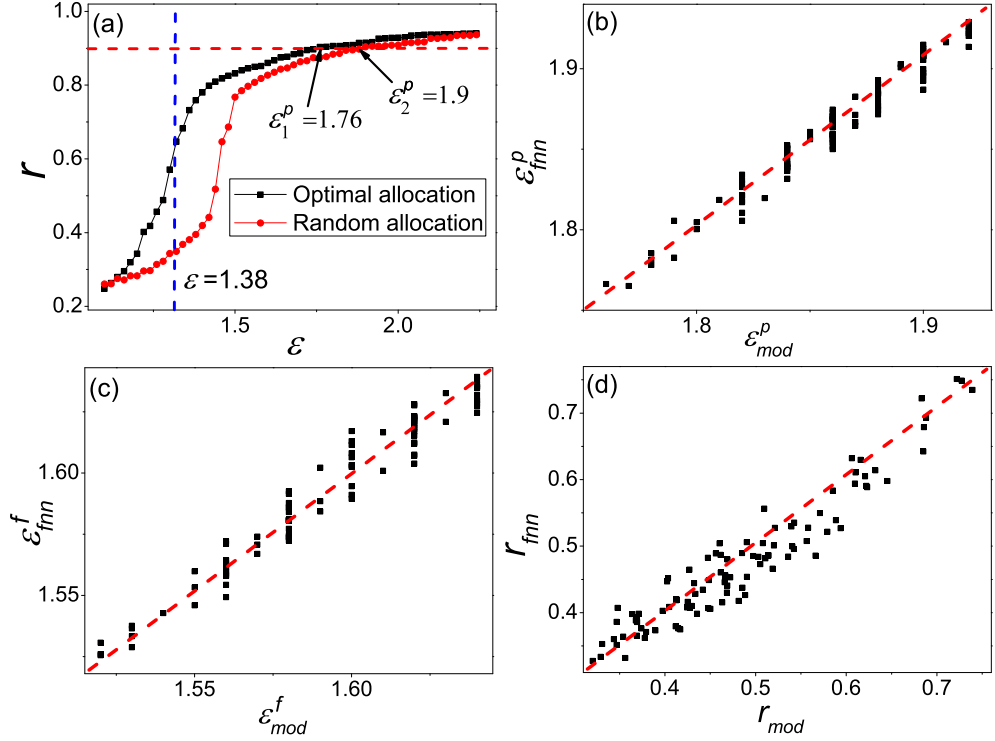

FIG. S3. *Inferring the synchronization of a scale-free network of size  $N = 100$ .* (a) The synchronization transitions for a random allocation scheme and the optimal allocation scheme identified by the machine. (b) Inference of the critical coupling,  $\varepsilon^p$ , for phase synchronization. (c) Inference of the critical coupling,  $\varepsilon^f$ , for frequency synchronization. (d) Inference of the synchronization order parameter under the intermediate coupling strength  $\varepsilon = 1.38$ . In (b-d), the red dashed lines denote the diagonal lines.

hub nodes). In optimizing the synchronization performance, only the ( $m$ ) chosen oscillators are allowed to exchange with each other, while the other oscillators are fixed on the network.

To infer the critical coupling for phase synchronization, we first generate  $\tilde{M} = 1000$  allocation schemes by random and then, by simulating the synchronization transition for each allocation scheme, obtain the data points  $(\Omega_l, \varepsilon_l^p)$ , with  $l = 1, \dots, \tilde{M}$ . As we did in the manuscript, phase synchronization is defined as the point where  $r > r_c = 0.9$ . The synchronization transition for a random allocation scheme is plotted in Fig. S3(a) (the red discs), which shows that  $\varepsilon^p \approx 1.9$  and  $r \approx 0.4$  at the intermediate coupling strength  $\varepsilon = 1.38$ . We use  $M = 700$  data points to train the machine, and use the remaining data points ( $M' = 300$ ) to optimize the hyperparameters. In inferring phase synchronization, the optimal hyperparameters are  $L = 1$  and  $n_1 = 100$ . The trained machine is then used to predict the critical couplings of phase synchronization for  $K = 1000$  new random allocations. Sampling results (100 in total) are given in Fig. S3(b), in which  $\varepsilon_{fnn}^p$  and  $\varepsilon_{mod}^p$  represent, respectively, the results predicted by the machine and the results obtained by model simulations. We see that the predictions are in good agreement with the true results. The averaged prediction error (averaged over  $K = 1000$  random allocations) is  $\langle e^p \rangle \approx 3.5 \times 10^{-3}$ .

In inferring the critical coupling for frequency synchronization, the measured data has the form  $(\Omega_l, \varepsilon_l^f)$ , with  $l = 1, \dots, \tilde{M}$  and  $\tilde{M} = 1200$ . The number of data points for training the model parameters is  $M = 800$ , and the remaining data points are used for optimizing the hyperparameters.

In this application, the hyperparameters are  $L = 2$  and  $(n_1, n_2) = (100, 10)$ . Sampling results are given in Fig. S3(c), in which  $\epsilon_{fnn}^f$  and  $\epsilon_{mod}^f$  represent, respectively, the results predicted by the machine and the results obtained by model simulations. The averaged prediction error (averaged over  $K = 1000$  allocations) is  $\langle e^f \rangle \approx 4 \times 10^{-3}$ .

In inferring the synchronization order parameter, the coupling strength is chosen as  $\epsilon = 1.38$  (within the regime of synchronization transition), and the total number of data points obtained based on the results of model simulations is  $\tilde{M} = 1500$  ( $M = 1000$  and  $M' = 500$ ). The optimal hyperparameters are  $L = 2$  and  $(n_1, n_2) = (100, 50)$ . Sampling results are given in Fig. S3(d). The averaged prediction error (averaged over  $K = 1000$  allocations) is  $\langle e \rangle_r \approx 6 \times 10^{-2}$ .

The synchronization performance of the optimal allocation (identified by the trained machine over  $K = 10000$  random allocations) is plotted in Fig. S3(a) (the black squares), which shows that phase synchronization is achieved at  $\epsilon^p \approx 1.76$ .

#### IV. RESULTS FOR NEPAL POWER-GRID

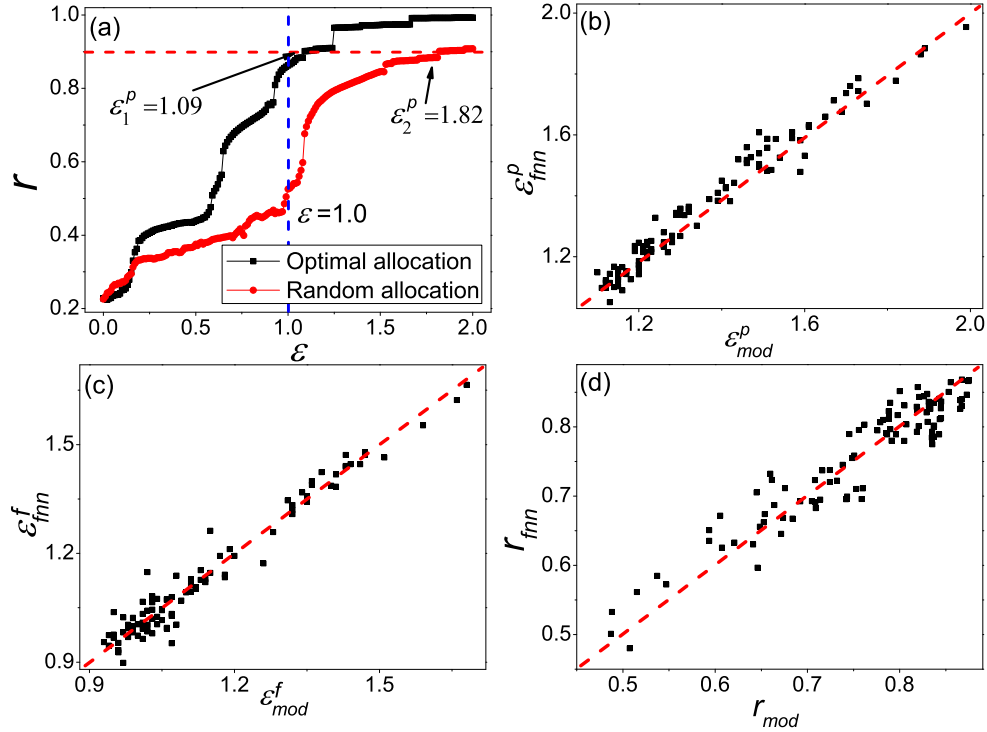

FIG. S4. *Inferring the synchronization of the Nepal power grid.* (a) Synchronization transitions for a random allocation scheme (red discs) and the optimal allocation scheme (black squares) identified by the machine. (b) Inference of the critical coupling,  $\epsilon^p$ , for phase synchronization. (c) Inference of the critical coupling,  $\epsilon^f$ , for frequency synchronization. (d) Inference of the synchronization order parameter under the intermediate coupling strength  $\epsilon = 1.0$ . In (b-d), the red dashed lines denote the diagonal lines.

The Nepal power grid contains  $N = 15$  nodes (power stations) and 62 links (transmission lines). The Nepal power grid is featured by the symmetric properties of the network structure, which affect significantly the network synchronization performance (see Ref. [27] in the manuscript for

more details). For simplicity, we still treat the network links as non-weighted and non-directed, i.e., the network structure is captured by an adjacency matrix. Again, the natural frequencies of the oscillators are chosen randomly from the range  $(-1, 1)$ . The synchronization transition of a random allocation scheme is plotted in Fig. S4(a) (the red discs), in which the critical coupling for phase synchronization is  $\epsilon^p \approx 1.82$  and  $r \approx 0.5$  at the intermediate coupling  $\epsilon = 1.0$ . For this small-size network, we are able to consider the scenario of unconstrained allocation, i.e., all  $N = 15$  oscillators are allowed to be relocated on the network by random.

In inferring phase synchronization, the measured dataset contains  $\tilde{M} = 1500$  points, among which  $M = 1000$  points are used for obtaining the model parameters and  $M' = 500$  points are used for optimizing the hyperparameters. The optimal hyperparameters are  $L = 1$  and  $n_1 = 25$ . The performance of the trained machine in inferring the phase synchronization of 100 random allocation schemes is plotted in Fig. S4(b). The averaged prediction error (averaged over  $K = 1000$  random allocations) is  $\langle e^p \rangle \approx 2.3 \times 10^{-2}$ . In inferring frequency synchronization, the measured data has the form  $(\Omega_i, \epsilon_i^f)$  and a total number of  $\tilde{M} = 1800$  data points are obtained based on the results of model simulations, among which  $M = 1400$  points are used in the training phase and  $M' = 400$  points are used in the validation phase. In this application, the hyperparameters are  $L = 2$  and  $(n_1, n_2) = (25, 10)$ . Sampling results are given in Fig. S4(c), in which  $\epsilon_{f_{nn}}^f$  and  $\epsilon_{f_{mod}}^f$  represent, respectively, the results predicted by the machine and the results obtained by model simulations. The averaged prediction error (averaged over  $K = 1000$  allocations) is  $\langle e^f \rangle \approx 3 \times 10^{-2}$ . In inferring the synchronization order parameter for the coupling strength  $\epsilon = 1.0$  (within the regime of synchronization transition), the total number of data points obtained by simulations is  $\tilde{M} = 2000$  ( $M = 1500$  and  $M' = 500$ ). The optimal hyperparameters are  $L = 2$  and  $(n_1, n_2) = (100, 50)$ . Sampling results are given in Fig. S4(d). The averaged prediction error (averaged over  $K = 1000$  allocations) is  $\langle e \rangle_r \approx 5 \times 10^{-2}$ .

The synchronization performance of the optimal allocation (identified by the trained machine among  $K = 10000$  random allocations) is plotted in Fig. S4(a) (the black squares), which shows that phase synchronization is achieved at  $\epsilon^p \approx 1.09$ . (The step-wise increase of  $r$  might be attributed to the symmetric properties of the network structure, which lead to the generation of different synchronization clusters in the transition to global synchronization. See Ref. [27] in the manuscript for details).

## V. RESULTS FOR CAT-BRAIN NETWORK

The cortical network of cat brain is adopted from Ref. [28] in the manuscript, which consists of  $N = 53$  nodes (brain areas) and 830 links (fiber connections). The cat-brain network is featured by the small-world feature and the community structures, which are new elements influencing the network synchronization performance. We still treat the links as non-weighted and non-directed (i.e., the network structure is captured by an adjacency matrix), and describe the nodal dynamics by heterogeneous phase oscillators whose natural frequencies are chosen randomly within the range  $(-1, 1)$ . The scenario of constrained allocation is considered here, with the number of relocatable oscillators being  $m = 10$ . The relocatable oscillators are chosen by random. The synchronization transition of a random allocation scheme is plotted in Fig. S5(a) (the red discs), in which the critical coupling for phase synchronization is  $\epsilon^p \approx 1.9$  and  $r \approx 0.5$  at the intermediate coupling  $\epsilon = 1.3$ . In inferring phase synchronization, the training dataset obtained from numerical simulations contains

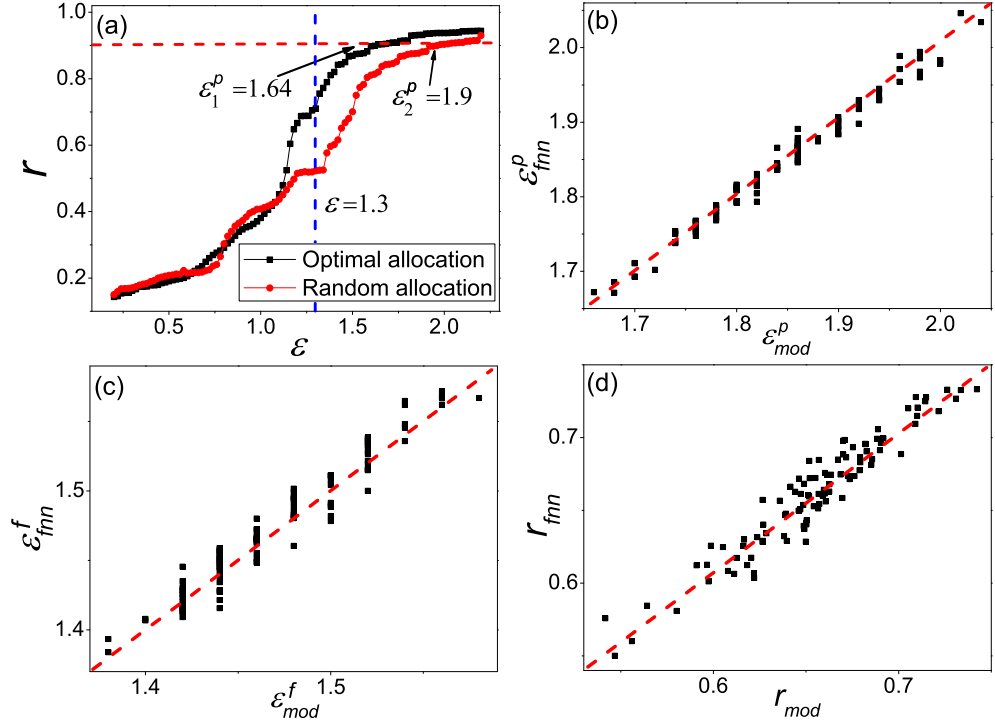

FIG. S5. *Inferring the synchronization of the cat-brain network.* (a) Synchronization transitions for a random allocation scheme (red discs) and the optimal allocation scheme (black squares) identified by the machine. (b) Inference of the critical coupling,  $\epsilon^p$ , for phase synchronization. (c) Inference of the critical coupling,  $\epsilon^f$ , for frequency synchronization. (d) Inference of the synchronization order parameter under the intermediate coupling strength  $\epsilon = 1.3$ . The red dashed lines in (b-d) denote the diagonal lines.

$\tilde{M} = 1200$  points, among which  $M = 800$  points are used for obtaining the model parameters and  $M' = 400$  points are used for optimizing the hyperparameters. The optimal hyperparameters are  $L = 1$  and  $n_1 = 50$ . The performance of the trained machine in inferring the phase synchronization of 100 random allocation schemes is plotted in Fig. S5(b). The averaged prediction error (averaged over  $K = 1000$  random allocations) is  $\langle e^p \rangle \approx 5 \times 10^{-3}$ .

In inferring the critical coupling for frequency synchronization, a total number  $\tilde{M} = 1700$  data points have been measured based on the results of model simulations, among which  $M = 1300$  points are used in the training phase and  $M' = 400$  points are used in the validation phase. Here the hyperparameters are  $L = 1$  and  $n_1 = 100$ . The performance of the trained machine in inferring the frequency synchronization of 100 random allocation schemes is plotted in Fig. S5(c). The averaged prediction error (averaged over  $K = 1000$  random allocations) is  $\langle e^f \rangle \approx 6 \times 10^{-3}$ . In inferring the synchronization order parameter of the intermediate coupling strength  $\epsilon = 1.3$ , the dataset contains  $\tilde{M} = 2000$  points ( $M = 1500$  and  $M' = 500$ ). The optimal hyperparameters are  $L = 1$  and  $n_1 = 100$ . Sampling results are shown in Fig. S5(d). The averaged prediction error (averaged over  $K = 1000$  allocations) is  $\langle e \rangle_r \approx 1.6 \times 10^{-2}$ .

The synchronization performance of the optimal allocation (identified by the trained machine among  $K = 10000$  random allocations) is plotted in Fig. S5(a) (the black squares), which shows that phase synchronization is achieved at  $\epsilon^p \approx 1.64$ .

## VI. RESULTS FOR NEMATODE NEURONAL NETWORK

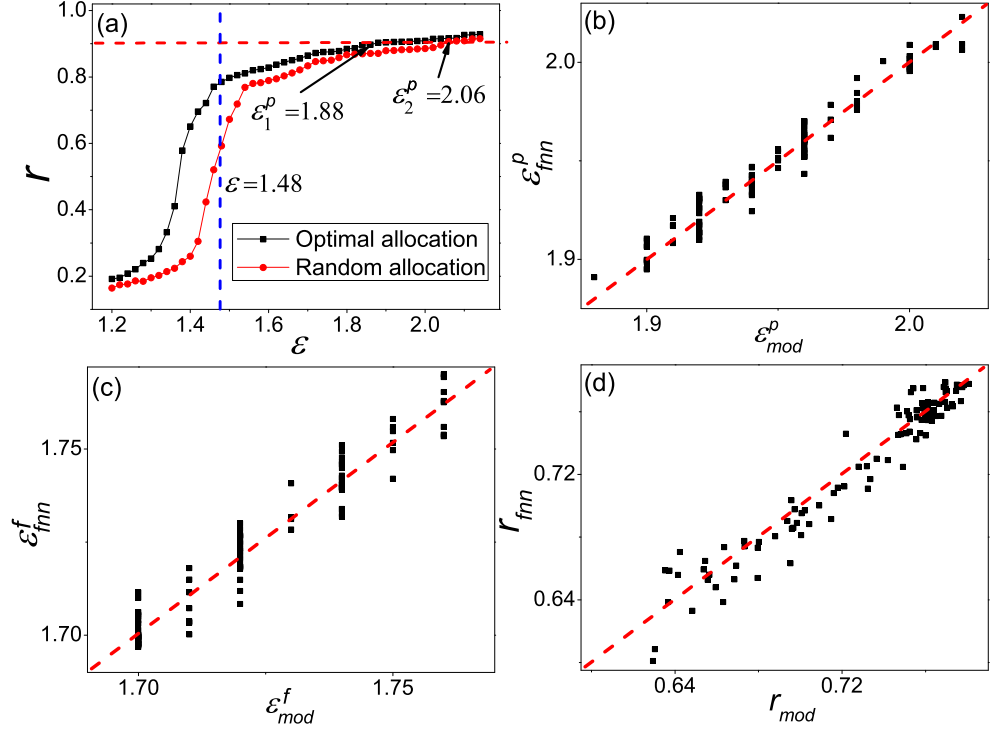

FIG. S6. *Inferring the synchronization of the Nematode neuronal network.* (a) Synchronization transitions for a random allocation scheme (red discs) and the optimal allocation scheme (black squares) identified by the machine. (b) Inference of the critical coupling,  $\epsilon^p$ , for phase synchronization. (c) Inference of the critical coupling,  $\epsilon^f$ , for frequency synchronization. (d) Inference of the synchronization order parameter under the intermediate coupling strength  $\epsilon = 1.48$ . The red dashed lines in (b-d) denote the diagonal lines.

The Nematode neuronal network is adopted from Ref. [29] in the manuscript, which contains  $N = 297$  neurons and 2345 links. Still, we adopt the Kuramoto model and consider the scenario of constrained allocation ( $m = 10$ ), with the relocatable oscillators being randomly chosen. In inferring phase synchronization, a total number of  $\tilde{M} = 2000$  random allocations have been simulated to obtain the training dataset, among which  $M = 1500$  data points are used to find the model parameters and  $M' = 500$  data points are used to find the optimal hyperparameters. The synchronization transition of a random allocation scheme is plotted in Fig. S6(a) (the red discs), in which the critical coupling for phase synchronization is  $\epsilon^p \approx 2.06$  and  $r \approx 0.6$  at the intermediate coupling  $\epsilon = 1.48$ . In inferring phase synchronization, the optimal hyperparameters are  $L = 2$  and  $(n_1, n_2) = (100, 50)$ .

The performance of the trained machine in inferring the phase synchronization of 100 random allocation schemes is plotted in Fig. S6(b). The averaged prediction error (averaged over  $K = 1000$  random allocations) is  $\langle e^p \rangle \approx 3.2 \times 10^{-3}$ .

In inferring the critical coupling for frequency synchronization, a total number  $\tilde{M} = 2200$  data points have been measured based on the results of numerical simulations, among which  $M = 1700$  points are used in the training phase and  $M' = 500$  points are used in the validation phase. Here the hyperparameters are  $L = 2$  and  $(n_1, n_2) = (100, 100)$ . The performance of the trained machine in

inferring the frequency synchronization of 100 random allocation schemes is plotted in Fig. S6(c). The averaged prediction error (averaged over  $K = 1000$  random allocations) is  $\langle e^f \rangle \approx 2.7 \times 10^{-3}$ . In inferring the synchronization order parameter for the coupling strength  $\epsilon = 1.48$ , the dataset contains  $\tilde{M} = 2500$  points ( $M = 2000$  and  $M' = 500$ ). The optimal hyperparameters are  $L = 2$  and  $(n_1, n_2) = (100, 200)$ . Sampling results are shown in Fig. S6(d). The averaged prediction error (averaged over  $K = 1000$  allocations) is  $\langle e \rangle_r \approx 1.7 \times 10^{-2}$ .

The synchronization performance of the optimal allocation (identified by the trained machine among  $K = 10000$  random allocations) is plotted in Fig. S6(a) (the black squares), which shows that phase synchronization is achieved at  $\epsilon^p \approx 1.88$ .

## VII. RESULTS FOR CHAOTIC RÖSSLER OSCILLATORS

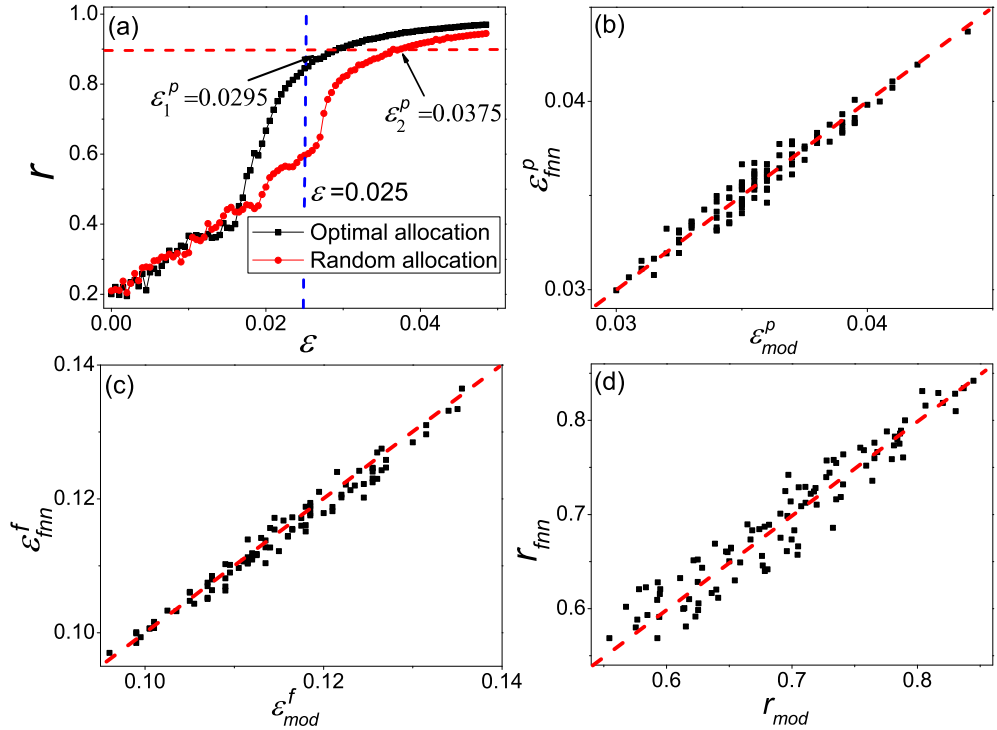

FIG. S7. *Inferring the synchronization of networked heterogeneous Rössler oscillators.* (a) Synchronization transitions for a random allocation scheme (red discs) and the optimal allocation scheme (black squares) identified by the machine. (b) Inference of the critical coupling,  $\epsilon^p$ , for phase synchronization. (c) Inference of the critical coupling,  $\epsilon^f$ , for frequency synchronization. (d) Inference of the synchronization order parameter under the intermediate coupling strength  $\epsilon = 0.025$ . The red dashed lines in (b-d) denote the diagonal lines.

The FNN technique is also capable of inferring the synchronization performance of networked heterogeneous chaotic oscillators. To demonstrate, we adopt the same random complex network studied in the manuscript ( $N = 20$  and  $p = 0.5$ ), but use heterogeneous chaotic Rössler oscillators

to describe the nodal dynamics. The system dynamics reads

$$\begin{aligned}\dot{x}_i &= -\omega_i y_i - z_i + \varepsilon \sum_{j=1}^N a_{ij}(x_j - x_i), \\ \dot{y}_i &= \omega_i x_i + 0.15 y_i, \\ \dot{z}_i &= 0.2 + z_i(x_i - 10),\end{aligned}\tag{S7.6}$$

where  $i = 1, \dots, N$  is the oscillator index,  $(x_i, y_i, z_i)$  denotes the state of oscillator  $i$ ,  $\mathbf{A} = \{a_{ij}\}$  is the adjacency matrix characterizing the network structure, and  $\omega_i$  the parameter governing the natural frequency of oscillator  $i$ . The value of  $\omega_i$  is randomly chosen within the range  $(0.9, 1.1)$ , and the motions of the isolated oscillators are chaotic. The synchronization degree is still characterized by the order parameter  $r = |\sum_j e^{i\theta_j}|/N$ ,  $j = 1, \dots, N$ , with  $\theta_j = \arctan(y_j/x_j)$  the instant phase of oscillator  $j$  (following Ref. [30] in the manuscript). Still, we consider the scenario of constrained allocation ( $m = 10$ ), with the relocatable oscillators being chosen randomly. In inferring phase synchronization, a total number of  $\tilde{M} = 2000$  random allocations have been simulated to obtain the training dataset, among which  $M = 1500$  data points are used to find the model parameters and  $M' = 500$  data points are used to find the optimal hyperparameters. The synchronization transition of a random allocation scheme is plotted in Fig. S7(a) (the red discs), in which the critical coupling for phase synchronization is  $\varepsilon^p \approx 0.0375$  and  $r \approx 0.6$  at  $\varepsilon = 0.025$ . In inferring phase synchronization, the optimal hyperparameters are  $L = 3$  and  $(n_1, n_2, n_3) = (50, 200, 50)$ . In this application, we adopt the hyperbolic tangent function (*Tanh*) as the activation function of the first hidden layer (so as to improve the sensitivity of the FNN to the input data), while the activation function of the other layers is still the *Relu* function.

The performance of the trained machine in inferring the phase synchronization of 100 random allocation schemes is plotted in Fig. S7(b). The averaged prediction error (averaged over  $K = 1000$  random allocations) is  $\langle e^p \rangle \approx 1.4 \times 10^{-2}$ .

In inferring the critical coupling for frequency synchronization, a total number  $\tilde{M} = 2200$  data points have been measured based on the results of numerical simulations, among which  $M = 1700$  points are used in the training phase and  $M' = 500$  points are used in the validation phase. Here the hyperparameters are  $L = 3$  and  $(n_1, n_2, n_3) = (50, 200, 100)$ . The performance of the trained machine in inferring the frequency synchronization of 100 random allocation schemes is plotted in Figs. S7(c). The averaged prediction error (averaged over  $K = 1000$  random allocations) is  $\langle e^f \rangle \approx 2.4 \times 10^{-2}$ . In inferring the synchronization order parameter for the coupling strength  $\varepsilon = 0.025$  (within the transition regime), the dataset contains  $\tilde{M} = 3000$  points ( $M = 2500$  and  $M' = 500$ ). The optimal hyperparameters are  $L = 3$  and  $(n_1, n_2, n_3) = (100, 200, 100)$ . Sampling results are shown in Fig. S7(d). The averaged prediction error (averaged over  $K = 1000$  allocations) is  $\langle e \rangle_r \approx 2.7 \times 10^{-2}$ .

The synchronization performance of the optimal allocation (identified by the trained machine among  $K = 10000$  random allocations) is plotted in Fig. S7(a) (the black squares), which shows that phase synchronization is achieved at  $\varepsilon^p \approx 0.0295$ .

## VIII. RESULTS FOR CHAOTIC FOODWEB OSCILLATORS

We finally exploit the FNN technique to infer the synchronization performance of a complex ecological network. The network structure is adopted from Ref. [31] in the manuscript, which

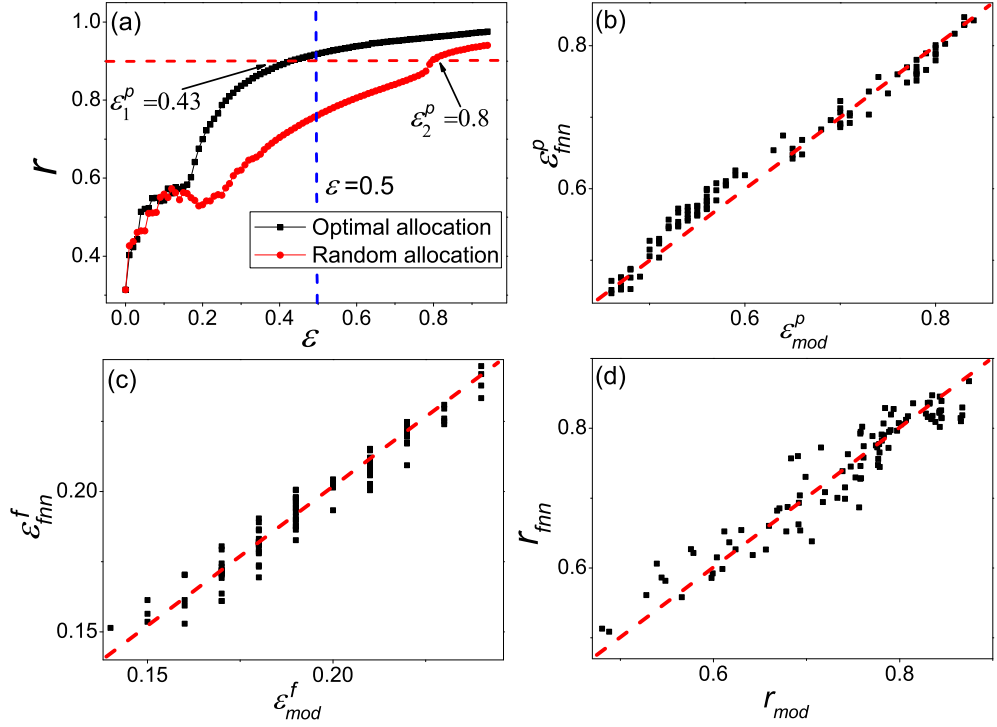

FIG. S8. *Inferring the synchronization of networked heterogeneous Foodweb oscillators.* (a) Synchronization transitions for a random allocation scheme (red discs) and the optimal allocation scheme (black squares) identified by the machine. (b) Inference of the critical coupling,  $\epsilon^p$ , for phase synchronization. (c) Inference of the critical coupling,  $\epsilon^f$ , for frequency synchronization. (d) Inference of the synchronization order parameter under the intermediate coupling strength  $\epsilon = 0.5$ . The red dashed lines in (b-d) denote the diagonal lines.

consists of  $N = 82$  nodes and 358 links. This network describes the habitat connections among animals in a riverine and estuarine ecosystem – an area of almost 580000ha and over 1400km of shoreline in the Coastal Plain of North Carolina. Here we use heterogenous foodweb oscillators (a vertical foodweb model showing the feature of uniform phase-growth and chaotic amplitude) to describe the nodal dynamics (see Ref. [32] in the manuscript for more details about this model). The network dynamics reads

$$\begin{aligned}
 \dot{x}_i &= \omega_i(x_i - x_0) - \alpha_1 x_i y_i + \epsilon \sum_{j=1}^N a_{ij}(x_j - x_i), \\
 \dot{y}_i &= -b y_i + \alpha_1 x_i y_i - \alpha_2 y_i z_i + \epsilon \sum_{j=1}^N a_{ij}(y_j - y_i), \\
 \dot{z}_i &= -c(z_i - z_0) + \alpha_2 y_i z_i + \epsilon \sum_{j=1}^N a_{ij}(z_j - z_i),
 \end{aligned} \tag{S8.7}$$

where  $i = 1, \dots, N$  is the oscillator index and  $\mathbf{A} = \{a_{ij}\}$  is the adjacency matrix characterizing the network structure. The nodal dynamics (the foodweb oscillator) is characterized by the set of parameters  $(\omega_i, \alpha_1, \alpha_2, b, c, x_0, z_0)$ . Here we fix  $(\alpha_1, \alpha_2, b, c, x_0, z_0) = (0.1, 0.6, 1, 10, 1.5, 0.01)$ , while the parameter  $\omega_i$  is chosen randomly from the range  $(0.95, 1.05)$ . The oscillators are chaotic in the isolated form, and, like the Rössler oscillator, the trajectory of each oscillator is rotating around the

origin in the phase space with a natural frequency characterized by the parameter  $\omega_i$ . This feature makes it possible to characterize the synchronization performance by the same order parameter,  $r$ , defined in the manuscript. Still, we consider the scenario of constrained allocation ( $m = 10$ ), with the relocatable oscillators being chosen randomly. A total number of  $\tilde{M} = 2500$  random allocations have been simulated to obtain the training dataset for inferring phase synchronization, among which  $M = 2000$  data points are used to find the model parameters and  $M' = 500$  data points are used to find the optimal hyperparameters. The synchronization transition of a random allocation scheme is plotted in Fig. S8(a) (the red discs), in which the critical coupling for phase synchronization is  $\epsilon^p \approx 0.8$  and  $r \approx 0.75$  at  $\epsilon = 0.5$ . In inferring phase synchronization, the optimal hyperparameters are  $L = 2$  and  $(n_1, n_2) = (50, 20)$ . As we did for the Rössler oscillators, we adopt the hyperbolic tangent function (*Tanh*) as the activation function for the first hidden layer, while the activation function of the other layers being still the *Relu* function.

The performance of the trained machine in inferring the phase synchronization of 100 random allocation schemes is plotted in Fig. S8(b). The averaged prediction error (averaged over  $K = 1000$  random allocations) is  $\langle e^p \rangle \approx 2.8 \times 10^{-2}$ .

In inferring the critical coupling for frequency synchronization, a total number of  $\tilde{M} = 2500$  data points have been measured based on the results of numerical simulations, among which  $M = 2000$  points are used in the training phase and  $M' = 500$  points are used in the validation phase. Here the hyperparameters are  $L = 3$  and  $(n_1, n_2, n_3) = (100, 150, 100)$ . The performance of the trained machine in inferring the frequency synchronization of 100 random allocation schemes is plotted in Fig. S8(c). The averaged prediction error (averaged over  $K = 1000$  random allocations) is  $\langle e^f \rangle \approx 2.9 \times 10^{-2}$ . In inferring the synchronization order parameter of the coupling strength  $\epsilon = 0.5$  (within the transition regime), the dataset contains  $\tilde{M} = 3000$  points ( $M = 2500$  and  $M' = 500$ ). The optimal hyperparameters are  $L = 3$  and  $(n_1, n_2, n_3) = (100, 200, 150)$ . Sampling results are shown in Fig. S8(d). The averaged prediction error (averaged over  $K = 1000$  allocations) is  $\langle e \rangle_r \approx 1.2 \times 10^{-2}$ .

The synchronization performance of the optimal allocation (identified by the trained machine among  $K = 10000$  random allocations) is plotted in Fig. S8(a) (the black squares), which shows that phase synchronization is achieved at  $\epsilon^p \approx 0.43$ .

## IX. INFERRING THE SYNCHRONIZATION PERFORMANCE OF A NEW SET OF OSCILLATORS

The machine trained by the set of oscillators with predefined natural frequencies can also be used to infer the synchronization of a new set of oscillators. To demonstrate, we adopt the network studied in Figs. 1 and 2 in the manuscript as the model, but selecting the natural frequencies of the  $m = 10$  relocatable oscillators by random within the range  $(-1, 1)$ . Using the machine that has been already trained by the data of the predefined oscillators, we anticipate the synchronization performance of the network for 100 new sets of oscillators, including the critical coupling strength for phase synchronization ( $\epsilon^p$ ), the critical coupling strength for frequency synchronization ( $\epsilon^f$ ), and the synchronization order parameter at a fixed coupling strength ( $\epsilon = 1.2$ ). The results are plotted in Fig. S9. We see that, despite the difference between the training and predicting sets, the results predicted by the machine are still in good agreement with the ones obtained by model simulations. The averaged errors (over 1000 predictions) are  $\langle e^p \rangle \approx 0.0189$ ,  $\langle e^f \rangle \approx 0.0237$  and

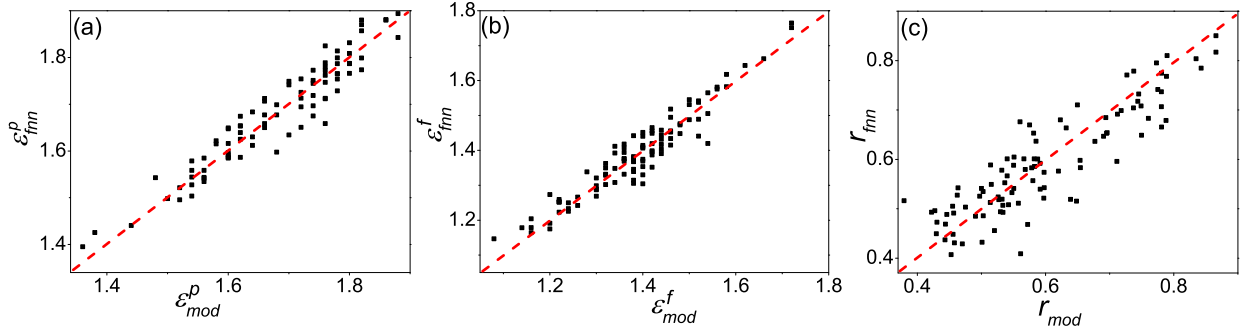

FIG. S9. *Using the trained machine to infer the synchronization performance of a different set of oscillators.* The network structure is the same as the one studied in the manuscript ( $N = 20$ ,  $p = 0.5$ ). The trained machine is used to predict the synchronization performance of 100 new sets of oscillators. In each prediction, the natural frequencies of the  $m = 10$  relocatable oscillators are chosen randomly from the range  $(-1, 1)$ . (a) Inference of phase synchronization. (b) Inference of frequency synchronization.  $\epsilon_{fm}$  and  $\epsilon_{mod}$  denote, respectively, the results predicted by the machine and by model simulations. (c) Inference of synchronization order parameter at coupling strength  $\epsilon = 1.2$ .  $r_{mod}$ : results obtained by model simulations.  $r_{fm}$ : results predicted by machine. Red dashed lines denote the diagonal lines.

$\langle e \rangle_{r=1.2} \approx 0.098$ , which are slightly worse than the results plotted in Fig. 2 in the manuscript.

## X. IMPACTS OF TRAINING DATA ON MACHINE PERFORMANCE

In evaluating the performance of any learning technique, an important issue concerns the generalization ability of the machine. That is, if the features (properties) of the training and testing data are different, will the trained machine being still able to predict the target system accurately? For the specific case studied in our present work, this question can be interpreted as follows: if the training data are collected from allocations clearly different from the optimal one, is it still possible to infer the optimal allocation by the machine? To address this question, we next conduct a statistical analysis on the properties of the training data, and investigate the impacts of the training data on the prediction performance of the machine by a data-tailoring strategy.

For the machine we have used for predicting the critical couplings,  $\epsilon^p$ , plotted in Fig. 2(a) in the manuscript, the training data are obtained by solving the dynamics of the network numerically (the ER network of  $N = 20$  nodes and  $m = 10$  relocatable oscillators). The training data contains  $\tilde{M} = 800$  data points of the form  $(\Omega, \epsilon^p)$ , with  $\Omega$  being a specific allocation scheme of the oscillators on the network and  $\epsilon^p$  being the associated critical coupling for achieving phase synchronization. Shown in Fig. S10(a) is the probability distribution of the critical couplings,  $\epsilon^p$ , for the training data. We see that the distribution is basically normal and the critical couplings are scattered within the range  $\epsilon^p \in [1.33, 1.96]$ . In particular, among all  $\tilde{M} = 800$  allocations generating the training data, the optimal allocation has the critical coupling  $\epsilon_{min}^p = 1.33$ . A check of the testing data (for  $K = 1000$  candidating allocations) plotted in Fig. 2(a) in the manuscript shows that the critical coupling of the testing data is also ranging from 1.33 to 1.96, which is completely overlapped with that of the training data. As such, the optimal allocation identified by the machine among the  $K = 1000$  testing allocations is already within the training set (or, if not exactly the same, is very

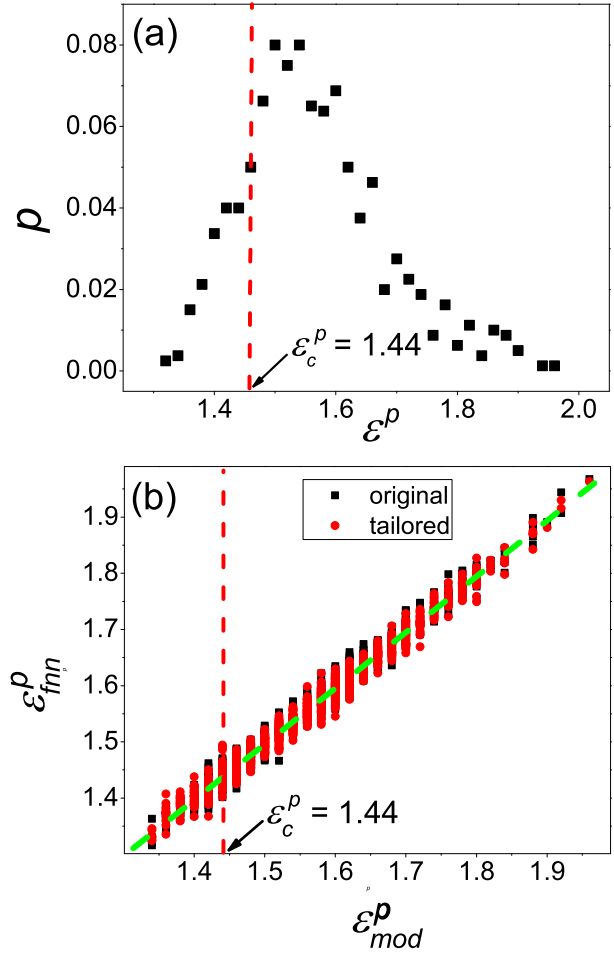

FIG. S10. *Impacts of training dataset on machine performance.* (a) Tailoring the training dataset. Shown is the distribution of the critical coupling,  $\epsilon^p$ , for  $\tilde{M} = 800$  data points that are obtained by model simulations and used for training the machine in the manuscript. Data points with  $\epsilon^p < \epsilon_c^p = 1.44$  are removed from the dataset. 100 data points are removed in total, and the tailored dataset contains  $\tilde{M} = 700$  data points. (b) Performance of the new machine trained by the tailored dataset. Black squares are results predicted by the machine trained by the original dataset. Red discs are results predicted by the new machine trained by the tailored dataset. It is seen that the new machine is able to anticipate the synchronization performance of the network outside the range of the training dataset, implying the generalization ability of the technique.

close to the optimal allocation in the training set). This raises the question about the generalization ability of the machine, as for large-size complex networks it is impossible to make sure that the training data cover the whole phase space (here it refers to the space of oscillator allocation). So, a check on the ability of generalization is necessary for the proposed technique.

We adopt a data-tailoring strategy to check the generalization ability of the machine. Specifically, by the ascending order of the critical coupling  $\epsilon^p$ , we remove from the training dataset (containing  $\tilde{M} = 800$  data points in total) 100 data points. This operation is to make sure that all allocations in the training dataset are clearly different from the optimal allocation. In the tailored dataset, the smallest coupling strength is  $\epsilon_c^p = 1.44$  [as depicted in Fig. S10(a)], which is clearly larger than that of the optimal allocation identified by the machine ( $\epsilon_{min}^p = 1.33$  for the  $K = 1000$

candidates studied in the present work). Our task here is to check whether the machine trained by the tailored dataset is still able to anticipate the synchronization performance of the allocations in the region below  $\epsilon_c^p$ . In doing this, we divide the data points ( $\tilde{M} = 700$  in total now) into two subsets,  $M = 450$  for the training phase and  $M' = 250$  for the validation phase. Following the same procedures described in the manuscript, we re-train the machine and then use the new machine to predict the synchronization performance of  $K = 1000$  allocations that are randomly generated (the same set of allocations that has been used in the manuscript for evaluating the machine performance). The results are plotted in Fig. S10(b) (red discs). We see that the new machine predicts the critical coupling accurately not only within the range of the training dataset,  $\epsilon^p \in [\epsilon_c^p, 1.96]$ , but also in the region below  $\epsilon_c^p$ . As a comparison, we plot in Fig. S10(b) also the results predicted by the machine that is trained by the original dataset ( $\tilde{M} = 800$ ) (black squares). It is seen that the results of the two machines are well overlapped. Specifically, both two machines predict that the optimal allocation (among 1000 candidates) is synchronized at about  $\epsilon_{min}^p \approx 1.33$ . To evaluate the overall performance of the new machine, we calculate the averaged predicting error defined in the manuscript,  $\langle e^p \rangle = \langle |1 - \epsilon_{fnn}^p / \epsilon_{mod}^p| \rangle$ . We have  $\langle e^p \rangle \approx 7.2 \times 10^{-3}$  for the new machine, which is slightly larger than the error of the original machine ( $\langle e^p \rangle \approx 7 \times 10^{-3}$ ). We attribute the difference to the reduced training dataset ( $\tilde{M} = 800$  for the original dataset and  $\tilde{M} = 700$  for the tailored dataset), as the machine is better trained by a larger dataset in general. The results in Fig. S10 imply that the machine trained by the tailored dataset is able to “sense” the synchronization performance of the network outside the training region, confirming thereby the generalization ability of the FNN technique.
